# Supplementary material for: Exploiting Semantic Scene Reconstruction for Estimating Building Envelope Characteristics
Source: arXiv:2410.22383 source file (2024-10-29)
Supplement: Supplementary file 1 [file appendix.tex]

\section*{Appendix}

\begin{table}[!ht]
    \centering
    \caption{Window-to-Wall Ratio Estimation on Photo-realistic Synthetic Building}
    \resizebox{1\columnwidth}{!}{
\begin{tabular}{cc|ccc|ccc|ccc|ccc}
\toprule
\multicolumn{2}{l}{\multirow{3}{*}{}} & \multicolumn{3}{c}{\textbf{Building 1}} & \multicolumn{3}{c}{\textbf{Building 2}} & \multicolumn{3}{c}{\textbf{Building3}} & \multicolumn{3}{c}{\textbf{Building 4}} \\
\multicolumn{2}{l}{} & WWR & Window Area  & Wall Area & WWR & Window Area  & Wall Area & WWR & Window Area  & Wall Area & WWR & Window Area  & Wall Area\\
\multirow{2}{*}{2D Semantics} & Ideal View & 0.082 & 0.319 & 0.258 & 0.058 & 0.168 & 0.104 & 0.422 & 0.505 & 0.143 & 0.184 & 0.487 & 0.256 \\
 & Multi View  & 0.086 & 0.318 & 0.253 & 0.085 & 0.214 & 0.119 & 0.476 & 0.553 & 0.147 & 0.135 & 0.419 & 0.250\\
 \cmidrule{1-14}
2D Semantics w/ & Ideal View & 0.073 & 0.167 & 0.102 & \textbf{0.011} & 0.084 & 0.094 & 0.265 & 0.314 & 0.067 & 0.051 & 0.067 & 0.015 \\
geometry constraint & Multi View & 0.069 & 0.161 & 0.100 & 0.023 & 0.075 & 0.095 & 0.319 & 0.364 & 0.065 & \textbf{0.006} & \textbf{0.024} & 0.017\\
\cmidrule{1-14}
Semantic-SDF & - & \textbf{0.000} & \textbf{0.005} & \textbf{0.005} & 0.038 & \textbf{0.026} & \textbf{0.011} & \textbf{0.063} & \textbf{0.070} & \textbf{0.008} & 0.040 & 0.032 & \textbf{0.008}  \\
\cmidrule{1-14}
Ground Truth & - & 0.135 & 62.18 & 462.26 & 0.146 & 199.82 & 1365.75 & 0.097 & 50.35 & 517.72 & 0.211 & 114.74 & 542.88\\
\bottomrule
\end{tabular}}
\end{table}
